# Supplementary material for: MonoPlane: Exploiting Monocular Geometric Cues for Generalizable 3D Plane Reconstruction
Source: arXiv:2411.01226 source file (2024-11-02)
Supplement: Supplementary file 1 [file table_supp.tex]

\begin{table*}[]
\caption{Single-view evaluation on indoor datasets ScanNet~\cite{dai2017scannet} and Matterport3D~\cite{chang2017matterport3d}.}
%We do not evaluate plane detection for PlaneRecover~\cite{yang2018recovering} since their method does not estimate a per-pixel depth map for the whole image.}
\centering
\resizebox{0.9\linewidth}{!}{
\begin{tabular}{lllllll}
\toprule
\centering
\multirow{2}{*}{Method / Metrics} & \multicolumn{3}{c}{Plane Segmentation Metrics} & \multicolumn{3}{c}{Plane Recall (depth)} \\ \cmidrule(r){2-7} 
                                  & VOI~(↓)   & RI~(↑)  & \multicolumn{1}{l}{SC~(↑)}  & @0.05m     & @0.1m   & @0.6m   \\ 
\midrule 
\multicolumn{7}{c}{ScanNet~\cite{dai2017scannet}} \\
\midrule
PlaneRCNN~(ScanNet)~\cite{liu2019planercnn} & 1.297 & 0.852 & 0.699 &  0.194 & 0.417 & 0.674\\
PlaneTR~(ScanNet)~\cite{tan2021planetr}  & 0.767 & 0.925 & 0.838 & 0.245 & 0.437 & 0.616\\
PlaneRecTR~(ScanNet, SSA)~\cite{shi2023planerectr} & 0.652 & 0.943 & 0.865  & 0.363 & 0.577 & 0.756 \\ 
PlaneRecover~(Synthia, SSA) ~\cite{yang2018recovering} & 2.517 & 0.639  & 0.400 &  - & - & -\\
Ours~(SSA)  &   1.172  &   0.878 & 0.724  & 0.223  &  0.435  &  0.640 \\
Ours~(Zoe, SSA) & 1.337 & 0.839 & 0.669 & 0.174 & 0.374 & 0.558\\

PlaneRCNN~(ScanNet, unaligned)~\cite{liu2019planercnn} & 1.297 & 0.852 & 0.699 &  0.12 & 0.288 & 0.662\\
PlaneTR~(ScanNet, unaligned)~\cite{tan2021planetr}  & 0.767 & 0.925  & 0.838  &  0.208 & 0.382 & 0.614\\

PlaneRCNN~(ScanNet, CRF)~\cite{liu2019planercnn} & 1.157 & 0.864 & 0.726 &  0.171 & 0.396 & 0.644\\
PlaneTR~(ScanNet, CRF)~\cite{tan2021planetr}  & 0.761 & 0.923  & 0.837  &  0.26 & 0.44 & 0.606\\
\midrule
PlaneTR~(ScanNet, SA)~\cite{tan2021planetr} & 0.761 & 0.923  & 0.837 & 0.272 & 0.455 & 0.614 \\
PlaneRCNN~(ScanNet, SA)~\cite{liu2019planercnn} & 1.297 & 0.852 & 0.699 &  0.188 & 0.388 & 0.668\\
PlaneRecTR~(ScanNet, SA)~\cite{shi2023planerectr} & 0.652 & 0.943 & 0.865  & 0.345  & 0.548 & 0.753 \\ 
\midrule
PlaneTR~(ScanNet, Metric)~\cite{tan2021planetr} & 0.761 & 0.923  & 0.837 & 0.208 & 0.382 & 0.614 \\
PlaneRCNN~(ScanNet, Metric)~\cite{liu2019planercnn} & 1.297 & 0.852 & 0.699 & 0.12 & 0.288 & 0.662\\
PlaneRecTR~(ScanNet, Metric)~\cite{shi2023planerectr} & 0.652 & 0.943 & 0.865  & 0.232 & 0.442 & 0.754 \\ 
\midrule
\multicolumn{7}{c}{Matterport3D~\cite{chang2017matterport3d}} \\
\midrule
PlaneRCNN~(ScanNet, SSA)~\cite{liu2019planercnn} & 1.826 & 0.837 & 0.585 &  0.023 & 0.082 & 0.388\\
PlaneTR~(ScanNet, SSA)~\cite{tan2021planetr}  & 1.553 & 0.846  & 0.610  &  0.019 & 0.056 & 0.223\\
PlaneRecover~(Synthia, SSA)~\cite{yang2018recovering} & 2.868 & 0.713 & 0.366 &  - & - & -\\
PlaneRecTR~(ScanNet, SSA)~\cite{shi2023planerectr} & 1.419 & 0.875 & 0.655 &  0.036 & 0.104 & 0.345\\
Ours~(SSA)  & \textbf{1.222}  &   \textbf{0.902}   & \textbf{0.700}   &   \textbf{0.084}   &  \textbf{0.210}  &  \textbf{0.502}\\
PlaneRCNN~(ScanNet, omnidata)~\cite{liu2019planercnn}  & 1.826 & 0.837 & 0.585  & 0.005  & 0.023 & 0.252 \\ 
PlaneTR~(ScanNet, omnidata)~\cite{tan2021planetr}  & 1.553 & 0.846  & 0.610  &  0.014 & 0.043 & 0.191\\
PlaneRCNN~(ScanNet, omnidata, gt aligned before eval)~\cite{liu2019planercnn}  & 1.826 & 0.837 & 0.585  & 0.023  & 0.08 & 0.373 \\ 
PlaneTR~(ScanNet, omnidata, gt aligned before eval)~\cite{tan2021planetr}  & 1.553 & 0.846  & 0.610  &  0.018 & 0.052 & 0.215\\
PlaneRCNN~(ScanNet, CRF)~\cite{liu2019planercnn}  & 1.707 & 0.835 & 0.601  & 0.016  & 0.067 & 0.35 \\ 
PlaneTR~(ScanNet, CRF)~\cite{tan2021planetr}  & 1.477 & 0.845  & 0.616  &  0.019 & 0.054 & 0.223\\
PlaneRCNN~(ScanNet, unaligned)~\cite{liu2019planercnn}  & 1.826 & 0.837 & 0.585  & 0.005  & 0.023 & 0.252 \\ 
PlaneTR~(ScanNet, unaligned)~\cite{tan2021planetr}  & 1.553 & 0.846 & 0.610  & 0.02  & 0.058 & 0.308 \\ 
\midrule
PlaneTR~(ScanNet, SA)~\cite{tan2021planetr}  & 1.553 & 0.846 & 0.610  & 0.027  & 0.068 & 0.22 \\ 
PlaneRCNN~(ScanNet, SA)~\cite{liu2019planercnn} & 1.826 & 0.837 & 0.585 &  0.027 & 0.084 & 0.367\\
PlaneRecTR~(ScanNet, SA)~\cite{shi2023planerectr} & 1.419 & 0.875 & 0.655 & 0.045 & 0.108 & 0.33\\
\midrule
PlaneRecTR~(ScanNet, Metric)~\cite{shi2023planerectr} & 1.419 & 0.875 & 0.655 & 0.023 & 0.055 & 0.262\\
PlaneRCNN~(ScanNet, Metric)~\cite{liu2019planercnn} & 1.826 & 0.837 & 0.585 &  0.02 & 0.058 & 0.309\\
\bottomrule
\end{tabular}}
\label{tab::singleview-merged}
\end{table*}
